# Supplementary material for: Searching with and against the stream: Levy or Brown?
Source: arXiv:1306.1181 ancillary file (2013-06-05)
Supplement: Supplementary file 1 [file SI.pdf]

# Supporting Material
# Searching with and against the stream: Levy or Brown?

Vladimir V. Palyulin,[1] Aleksei V. Chechkin,[2,3] and Ralf Metzler[1,4]

[1]*Institute for Physics & Astronomy, University of Potsdam, D-14476 Potsdam-Golm, Germany*
[2]*Akhiezer Institute for Theoretical Physics NSC KIPT, Kharkov 61108, Ukraine*
[3]*Max Planck Institute for the Physics of Complex Systems, D-01187 Dresden, Germany*
[4]*Physics Department, Tampere University of Technology, FI-33101 Tampere, Finland*

(Dated: 5th June 2013)

We here present some supporting information on the dimensionless form of the dynamic equation of the biased Lévy flight process and the result for the first arrival density in the limit of a small bias. Moreover, we introduce the Fox $H$-function and discuss the non-monotonicity of the success probability $P$ to eventually locate the target.

## I. RESCALING OF DYNAMIC EQUATIONS

First arrival processes may be described by a $\delta$-sink with coefficient $\wp_{\mathrm{fa}}(t)$ in the corresponding fractional Fokker-Planck equation [1]. The density function $f(x,t)$ is then described by the dynamic equation

$$\frac{\partial f(x,t)}{\partial t} = K_\alpha \frac{\partial^\alpha f(x,t)}{\partial |x|^\alpha} - v\frac{\partial f(x,t)}{\partial x} - \wp_{fa}(t)\delta(x), \quad \text{(S1)}$$

where $K_\alpha$ is the generalized diffusion constant of physical dimension $\mathrm{cm}^\alpha/\mathrm{sec}$ [2]. Without loss of generality we place the target at $x=0$. To truthfully compare the search efficiency for different $\alpha$ values, in the main text we analyze the dimensionless version of the dynamic equation (S1). We introduce a length scale $\sigma$, which naturally arises from the scaling factor in the Lévy stable jump length distribution $\lambda(x)$, whose characteristic function reads

$$\mathcal{F}(\lambda(x)) = \int_{-\infty}^{\infty} e^{ikx}\lambda(x)dx = \exp\left(-\sigma^\alpha |k|^\alpha\right). \quad \text{(S2)}$$

A time scale is set by $\sigma^\alpha/K_\alpha$. We then introduce the dimensionless variables for time $K_\alpha t/\sigma^\alpha$ and space $x/\sigma$ to arrive at Eq. (1) of the main text. In terms of these units the discretized Langevin equation reads

$$x_{n+1} - x_n = -v\delta t + (\delta t)^{1/\alpha}\,\xi_{\alpha,1}(n), \quad \text{(S3)}$$

where $\xi_{\alpha,1}(n)$ is a set of random variables with Lévy stable distribution following the characteristic function (S2). In order to simulate normalized Lévy stable distributions we used the distribution generators from Ref. [3].

## II. TARGET SIZE IN THE SIMULATIONS

Although the theoretical approach to first arrival rests on a point sink, in simulations we consider a small yet finite target. The exact choice of this target size needs some care. We checked whether a target is sufficiently large by comparison of the simulation results for the tails of the arrival density with the limiting results of Ref. [1] in the case case without drift, namely, $\wp_{fa}(t) \simeq C(\alpha)\frac{x_0^{\alpha-1}}{t^{2-1/\alpha}}$, where $C(\alpha)$ is defined above. The results are shown in Fig. S1. If the target size increases, the power-law scaling for a point-like target $[\wp_{fa}(t) \sim t^{-2+1/\alpha}]$ crosses over to the Sparre-Andersen law $\wp_{fa}(t) \sim t^{-3/2}$ for the first passage across a target, as demonstrated in Fig. S2.

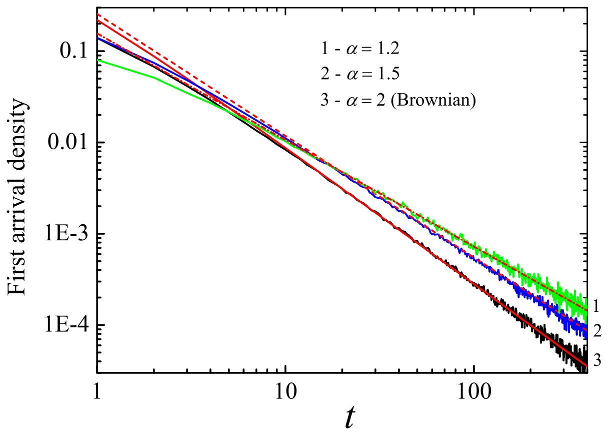


Figure S1: First arrival density from simulations of unbiased LFs for various $\alpha$ and initial position $x_0 = 1.0$. The colored curves denote simulation results. The superimposed red lines correspond to the analytical limiting laws ($\wp_{fa}(t) \sim t^{-2+1/\alpha}$). The target sizes were chosen as 0.01 for $\alpha = 2$; 1.5 and 0.0005 for $\alpha = 1.2$.

## III. FIRST ARRIVAL IN SMALL BIAS LIMIT

In case of a weak bias $|v| \ll 1$ we expand Eq. (2) in a series in powers of $v$. To first order, we obtain the result

$$\wp_{\mathrm{fa}}(s) = \frac{\sqrt{\pi}}{2\Gamma}\left(H^{12}_{31}\left[z\,\middle|\,\begin{matrix}\left(1,\frac{1}{2}\right),\left(\frac{1}{\alpha},\frac{1}{\alpha}\right),\left(\frac{1}{2},\frac{1}{2}\right)\\ \left(\frac{1}{\alpha},\frac{1}{\alpha}\right)\end{matrix}\right]\right.$$
$$\left. -2^{2-\alpha}\mathrm{Pe}_\alpha H^{12}_{31}\left[z\,\middle|\,\begin{matrix}\left(\frac{\alpha}{2},\frac{1}{2}\right),\left(\frac{1}{\alpha},\frac{1}{\alpha}\right),\left(\frac{\alpha+1}{2},\frac{1}{2}\right)\\ \left(\frac{\alpha+1}{\alpha},\frac{1}{\alpha}\right)\end{matrix}\right]\right) \quad \text{(S4)}$$

in terms of an $H$-function (see below), with $z = 2\left(sx_0^\alpha\right)^{-1/\alpha}$, $\Gamma = \Gamma(1/\alpha)\Gamma(1-1/\alpha)$, and the generalized

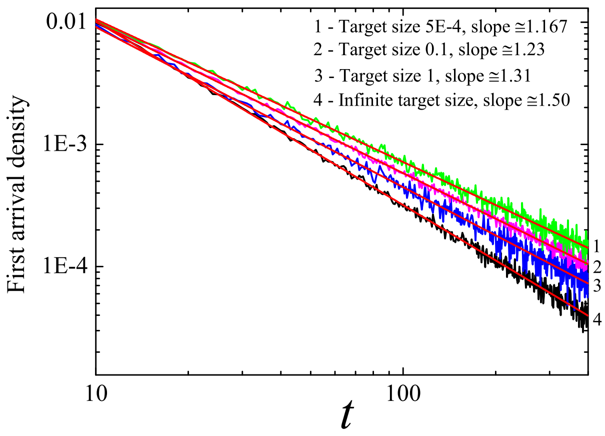


Figure S2: Same as Fig. S1, for the indicated parameters.

Péclet number $\mathrm{Pe}_\alpha = v x_0^{\alpha-1}/2$. For $\alpha = 2$ Eq (S4) reproduces the known Brownian result at small Pe, $\wp_{\mathrm{fa}}(t) \sim (1-\mathrm{Pe}) x_0 e^{-x_0^2/(4t)}/(4\pi t^3)^{1/2}$ [4]. In absence of a bias ($\mathrm{Pe}_\alpha = 0$), Tauberian theorems lead to the asymptotic behavior $\wp_{\mathrm{fa}}(t) \simeq C(\alpha) x_0^{\alpha-1} t^{1/\alpha-2}$ for the first passage density, where $C(\alpha) = \pi^{-2}\alpha \sin^2(\pi/\alpha)\sin(\pi(2-\alpha)/2)/(\alpha-1)\Gamma(2-\alpha)\Gamma(2-1/\alpha)$, which matches an earlier result [1]. The consequences of result (S4) are discussed in the context of the efficiency $\mathcal{E}$ in the main text.

To obtain expression (S4) from the general Laplace space solution for $\wp_{\mathrm{fa}}$ we used the generic formulas for $H$-functions, see Refs. [6]. Expansion of Eq. (2) up to first order reads

$$\wp_{\mathrm{fa}}(s) \simeq \frac{\int_{-\infty}^{\infty} \xi^{-1}\cos k dk - \int_{-\infty}^{\infty} 2\xi^{-1}\mathrm{Pe}_\alpha k \sin k dk}{\int_{-\infty}^{\infty} \xi^{-1} dk} \tag{S5}$$

where $\xi = s x_0^\alpha + |k|^\alpha$. With the identity [6]

$$\frac{1}{1+y^\alpha} = H_{11}^{11}\left[ y \left| \begin{matrix} (0, 1/\alpha) \\ (0, 1/\alpha) \end{matrix} \right. \right] \tag{S6}$$

the integrals in the expansion can be computed in terms of $H$-functions. For instance,

$$\int_{-\infty}^{\infty} \frac{\cos k}{\xi} dk = 2(s x_0^\alpha)^{\frac{1-\alpha}{\alpha}} \int_0^\infty \cos\left(s^{1/\alpha} x_0 y\right) H_{11}^{11}\left[ y \left| \begin{matrix} (0, \frac{1}{\alpha}) \\ (0, \frac{1}{\alpha}) \end{matrix} \right. \right] dy = \frac{2\sqrt{\pi}}{\alpha s x_0^\alpha} H_{31}^{12}\left[ \frac{2}{s^{1/\alpha} x_0} \left| \begin{matrix} \left(\frac{1}{2}, \frac{1}{2}\right), \left(0, \frac{1}{\alpha}\right), \left(0, \frac{1}{2}\right) \\ \left(0, \frac{1}{\alpha}\right) \end{matrix} \right. \right] \tag{S7}$$

or

$$\int_{-\infty}^{\infty} \frac{2\mathrm{Pe}_\alpha \sin k}{\xi^2} dk = 4\mathrm{Pe}_\alpha \left(s x_0^\alpha\right)^{\frac{2}{\alpha}-2} \int_0^\infty \frac{y \sin\left(s^{1/\alpha} x_0 y\right)}{1+y^\alpha} dy = \frac{8\mathrm{Pe}_\alpha \sqrt{\pi}}{\alpha \left(s x_0^\alpha\right)^2} H_{31}^{12}\left[ \frac{2}{s^{1/\alpha} x_0} \left| \begin{matrix} \left(-\frac{1}{2}, \frac{1}{2}\right), \left(-1, \frac{1}{\alpha}\right), \left(0, \frac{1}{2}\right) \\ \left(0, \frac{1}{\alpha}\right) \end{matrix} \right. \right] \tag{S8}$$

The integral in the denominator of (S5) can be found in integral tables [5]. Thus, we obtain expression (S4).


[1] A. V. Chechkin, R. Metzler, V. Yu. Gonchar, J. Klafter and L. V. Tanatarov, J. Phys. A **36**, L537 (2003).
[2] R. Metzler and J. Klafter, Phys. Rep. **339**, 1 (2000).
[3] J. M. Chambers, C. L. Mallows, B. W. Stuck, J. Amer. Statist. Assoc. **71**, 340 (1976).
[4] S. Redner, A Guide to First-Passage Processes (Cambridge University Press, Cambridge, UK, 2001).
[5] A. P. Prudnikov, Y. A. Brychkov, O. I. Marichev, Integrals and series (Gordon and Breach Science, New York, 1990).
[6] A.M. Mathai, R.K. Saxena and H.J. Haubold, The H-Function Theory and Applications (Springer 2010).
